# Supplementary material for: Anomalous diamagnetic response in multi-band superconductors with time-reversal broken symmetry
Source: arXiv:1707.02345 source file (2017-07-07)
Supplement: Supplementary file 1 [file Supplemental.pdf]

# Supplemental material for “Anomalous diamagnetic response in multi-band superconductors with time-reversal broken symmetry”

Yuriy Yerin
B. Verkin Institute for Low Temperature Physics and Engineering, National Academy of Sciences of Ukraine, 47 Lenin Ave., 61103, Kharkiv, Ukraine
Institute for Physics of Microstructures, Russian Academy of Sciences, 603590 Nizhny Novgorod, GSP 105, Russia

Alexander Omelyanchouk
B. Verkin Institute for Low Temperature Physics and Engineering, National Academy of Sciences of Ukraine, 47 Lenin Ave., 61103, Kharkiv, Ukraine

Stefan-Ludwig Drechsler, Dmitri V. Efremov, and Jeroen van den Brink
Institute for Theoretical Solid State Physics, Leibniz-Institut für Festkörper- und Werkstoffforschung IFW-Dresden, D-01169 Dresden, Helmholtzstraße 20, Germany

## 1. Equilibrium non-current states in a three-band superconductor

The simplest form of a Ginzburg-Landau (GL) free energy density for three-band superconductors including the fundamental interband interactions, can be written in the following form

$$F = \sum_{i=1}^{3} F_i - F_{\text{int}}, \tag{S1}$$

where $F_i$ are the standard direct intraband contributions from each of the band related order parameters

$$F_i = \alpha_i \left|\psi_i\right|^2 + \frac{1}{2}\beta_i \left|\psi_i\right|^4 + \frac{1}{2m_i}\left|\left(-i\hbar\nabla - \frac{2e}{c}\mathbf{A}\right)\psi_i\right|^2 , \tag{S2}$$

and $F_{\text{int}}$ is the interaction term of the functional, which describes the phase sensitive Josephson-like interband coupling of the order parameters and the usual interband scattering

$$F_{\text{int}} = \gamma_{12}\left(\psi_1^*\psi_2 + \psi_1\psi_2^*\right) + \gamma_{13}\left(\psi_1^*\psi_3 + \psi_3\psi_1^*\right) + \gamma_{23}\left(\psi_2^*\psi_3 + \psi_2\psi_3^*\right) \tag{S3}$$

Here $\gamma_{ij}$ are the interaction coefficients, which can be positive or negative. It’s important to note that for two-band superconductors with a given negative sign in front of the interaction term in Eq. (S1) corresponds to a ground state with zero phase difference between the order two parameters when $\gamma > 0$, while it is changed to π when $\gamma < 0$. So we keep the same sign convention in $F_{\text{int}}$ for the three-band superconductors considered here, too.

First of all in order to understand what kind of phase differences are realized in the homogeneous and equilibrium state of a three-band superconductor, we look for the minimum of its free energy GL functional. We rewrite Eq. (S1) in terms of the order parameter moduli and phase differences $\psi_i = \left|\psi_i\right|\exp\left(i\varphi_i\right)$, where $i$=1, 2, 3 and introduce the phase-variables

$$\varphi_1 - \varphi_2 = \phi, \tag{S4}$$

$$\varphi_1 - \varphi_3 = \theta. \tag{S5}$$

Then we are left with two phase-variables, only:

$$F = \sum_{i=1}^{3} F_i - 2\gamma_{12}|\psi_1||\psi_2|\cos\phi - 2\gamma_{13}|\psi_1||\psi_3|\cos\theta - 2\gamma_{23}|\psi_2||\psi_3|\cos(\theta-\phi). \tag{S6}$$

Obviously, a minimum of the GL free energy density will occur, if the interaction term $F_{\text{int}}$ has a maximum. So below we will focus on this term considering it as a function of the two new phase-variables, i.e. $F_{\text{int}} = F_{\text{int}}(\phi,\theta)$.

To shorten our notation we measure the interaction energy in units of $2|\gamma_{23}||\psi_2||\psi_3|$ and then introduce:

$$G_1 = \frac{\gamma_{12}}{|\gamma_{23}|}\frac{|\psi_1|}{|\psi_3|},\ G_2 = \operatorname{sgn}(\gamma_{23}),\text{ and } G_3 = \frac{\gamma_{13}}{|\gamma_{23}|}\frac{|\psi_1|}{|\psi_2|}. \tag{S7}$$

The conditions for an extremum of $F_{\text{int}}(\phi,\theta)$ yield the two equations:

$$-G_1\sin\phi + G_2\sin(\theta-\phi) = 0, \tag{S8}$$

$$-G_3\sin\theta - G_2\sin(\theta-\phi) = 0. \tag{S9}$$

Eqs. (S8) and (S9) must be supplemented by the equilibrium GL equations for the amplitudes for the three order parameters

$$\alpha_1|\psi_1| + \beta_1|\psi_1|^3 - \gamma_{12}|\psi_2|\cos\phi - \gamma_{13}|\psi_3|\cos\theta = 0, \tag{S10}$$

$$\alpha_2|\psi_2| + \beta_2|\psi_2|^3 - \gamma_{12}|\psi_1|\cos\phi - \gamma_{23}|\psi_3|\cos(\theta-\phi) = 0, \tag{S11}$$

$$\alpha_3|\psi_3| + \beta_3|\psi_3|^3 - \gamma_{13}|\psi_1|\cos\theta - \gamma_{23}|\psi_2|\cos(\theta-\phi) = 0. \tag{S12}$$

Thus, in total we have five equations (S8)-(S12), which in particular determine the extremal values (maximum, saddle and minimum points) of $\phi$ and $\theta$ we are looking for.

The solutions of Eqs. (S8)-(S12) for $\phi$ and $\theta$ depend on their arrangement in each of the four quadrants.

In particular, introducing $\Omega = \sqrt{1 - \frac{1}{4}\left[\left(G_1^2G_3^2 + G_1^2 - G_3^2\right)/\left(G_1^2G_2G_3\right)\right]^2}$

for $\phi \in [0,\pi]$ and $\theta \in [0,\pi]$ we have:

$$\begin{cases}\phi = \arcsin\Omega, \\ \theta = \arcsin\left(\left|\frac{G_1}{G_3}\right|\Omega\right),\end{cases} \quad \begin{cases}\phi = \pi - \arcsin\Omega, \\ \theta = \pi - \arcsin\left(\left|\frac{G_1}{G_3}\right|\Omega\right),\end{cases} \tag{S13}$$

Thereby at the origin of that quadrant $\begin{cases}\phi = 0, \\ \theta = 0,\end{cases}$ is fulfilled, (S14)

whereas for $\phi \in [\pi, 2\pi]$ and $\theta \in [0, \pi]$

$$\begin{cases} \phi = 2\pi - \arcsin \Omega, \\ \theta = \arcsin\left(\left|\frac{G_1}{G_3}\right|\Omega\right), \end{cases} \quad \begin{cases} \phi = \pi + \arcsin \Omega, \\ \theta = \pi - \arcsin\left(\left|\frac{G_1}{G_3}\right|\Omega\right), \end{cases} \qquad \text{(S15)}$$

At the origin of the second quadrant $\begin{cases} \phi = \pi, \\ \theta = 0, \end{cases}$ is obeyed, (S16)

furthermore for the third quadrant $\phi \in [0, \pi]$ and $\theta \in [\pi, 2\pi]$ we have:

$$\begin{cases} \phi = \arcsin \Omega, \\ \theta = 2\pi - \arcsin\left(\left|\frac{G_1}{G_3}\right|\Omega\right), \end{cases} \quad \begin{cases} \phi = \pi - \arcsin \Omega, \\ \theta = \pi + \arcsin\left(\left|\frac{G_1}{G_3}\right|\Omega\right), \end{cases} \qquad \text{(S17)}$$

and at its origin $\begin{cases} \phi = 0, \\ \theta = \pi, \end{cases}$ holds, (S18)

and finally for the fourth quadrant $\phi \in [\pi, 2\pi]$ and $\theta \in [\pi, 2\pi]$ we have:

$$\begin{cases} \phi = 2\pi - \arcsin \Omega, \\ \theta = 2\pi - \arcsin\left(\left|\frac{G_1}{G_3}\right|\Omega\right), \end{cases} \quad \begin{cases} \phi = \pi + \arcsin \Omega, \\ \theta = \pi + \arcsin\left(\left|\frac{G_1}{G_3}\right|\Omega\right), \end{cases} \qquad \text{(S19)}$$

where at its origin $\begin{cases} \phi = \pi, \\ \theta = \pi. \end{cases}$ is obeyed. (S20)

The selection of the corresponding solutions for a given $G_i$ is determined by a special system of inequalities, following from the stability condition for the maximum of $F_{\text{int}}$ (see Eq. (21))

$$\begin{cases} \dfrac{\partial^2 F_{\text{int}}}{\partial \phi^2} < 0, \\ \dfrac{\partial^2 F_{\text{int}}}{\partial \phi^2} \cdot \dfrac{\partial^2 F_{\text{int}}}{\partial \theta^2} - \left(\dfrac{\partial^2 F_{\text{int}}}{\partial \phi \partial \theta}\right)^2 > 0. \end{cases} \qquad \text{(S21)}$$

The ratios $|\psi_1|/|\psi_3|$ and $|\psi_1|/|\psi_2|$, being a part of $G_1$ and $G_3$, can be found after substituting the expressions (S13)-(S20) into Eqs. (S10)-(S12) and from their solutions. Next, the obtained solutions have to be inserted into Eqs. (S13)-(S20). As a result finally we arrive at final expressions for $\phi$ and $\theta$.

The selection of the corresponding solutions for given $G_i$ is determined by a special system of inequalities, following from the stability condition for the maximum of $F_{\text{int}}$.

In Fig. S1 we show first explicitly the border lines for the BTRS-states in a particular range of parameters ($G_1 < 0, G_2 = 1, G_3 > 0$):

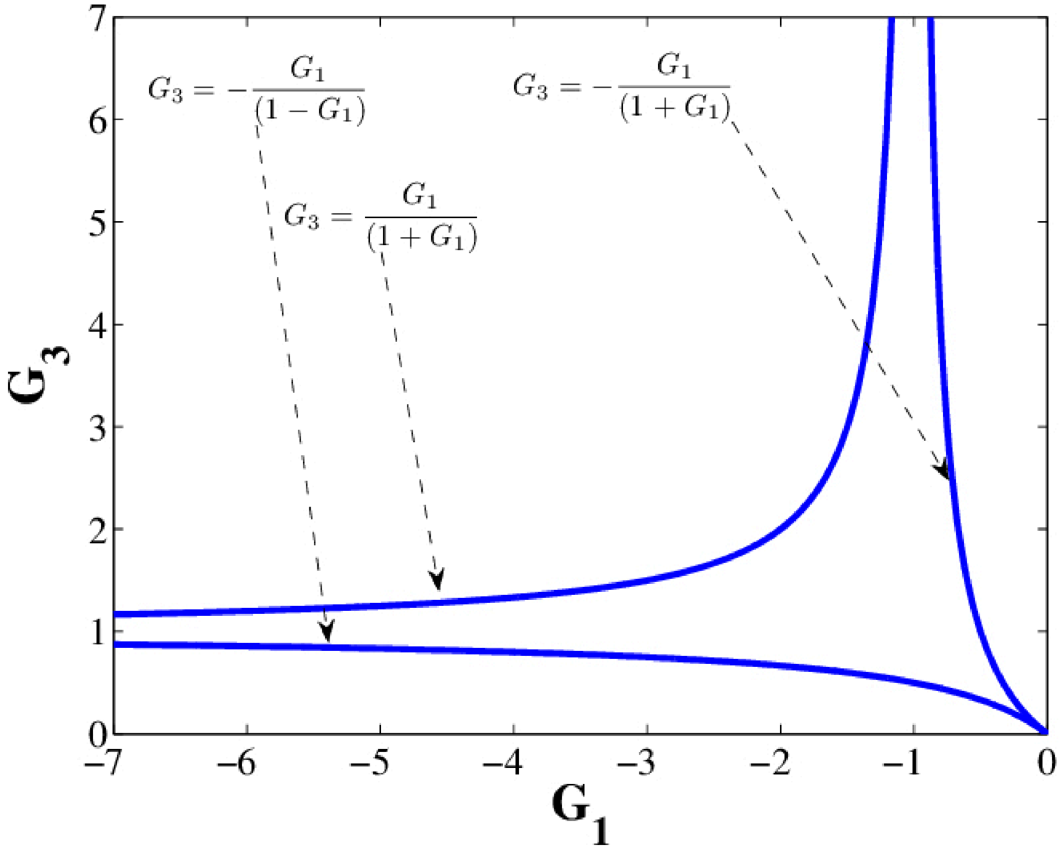


Fig. S1. Border lines of one of the BTRS-regions (inside the central area restricted by the blue lines). Notice the continuation of each of these phases with interchanged areas in the corresponding other region e.g. ($G_1 > 0, G_3 < 0$) (see also Figs. S2 and S3).

The analytic expressions for the blue curves, which limit the BTRS area have been found from the stability conditions

$$\begin{cases} \dfrac{\partial^2 F_{\text{int}}}{\partial \phi^2} < 0, \\ \dfrac{\partial^2 F_{\text{int}}}{\partial \phi^2} \cdot \dfrac{\partial^2 F_{\text{int}}}{\partial \theta^2} - \left( \dfrac{\partial^2 F_{\text{int}}}{\partial \phi \partial \theta} \right)^2 > 0. \end{cases} \tag{S21}$$

Based on Eqs. (S10-S20) and the stability conditions (S21), we depict graphically the allowed values of the phase-differences in dependence on $G_1$ and $G_3$ for $G_2 = 1$ (Fig. S2) and $G_2 = -1$ (Fig. S3) and Fig. 2 in the main text.

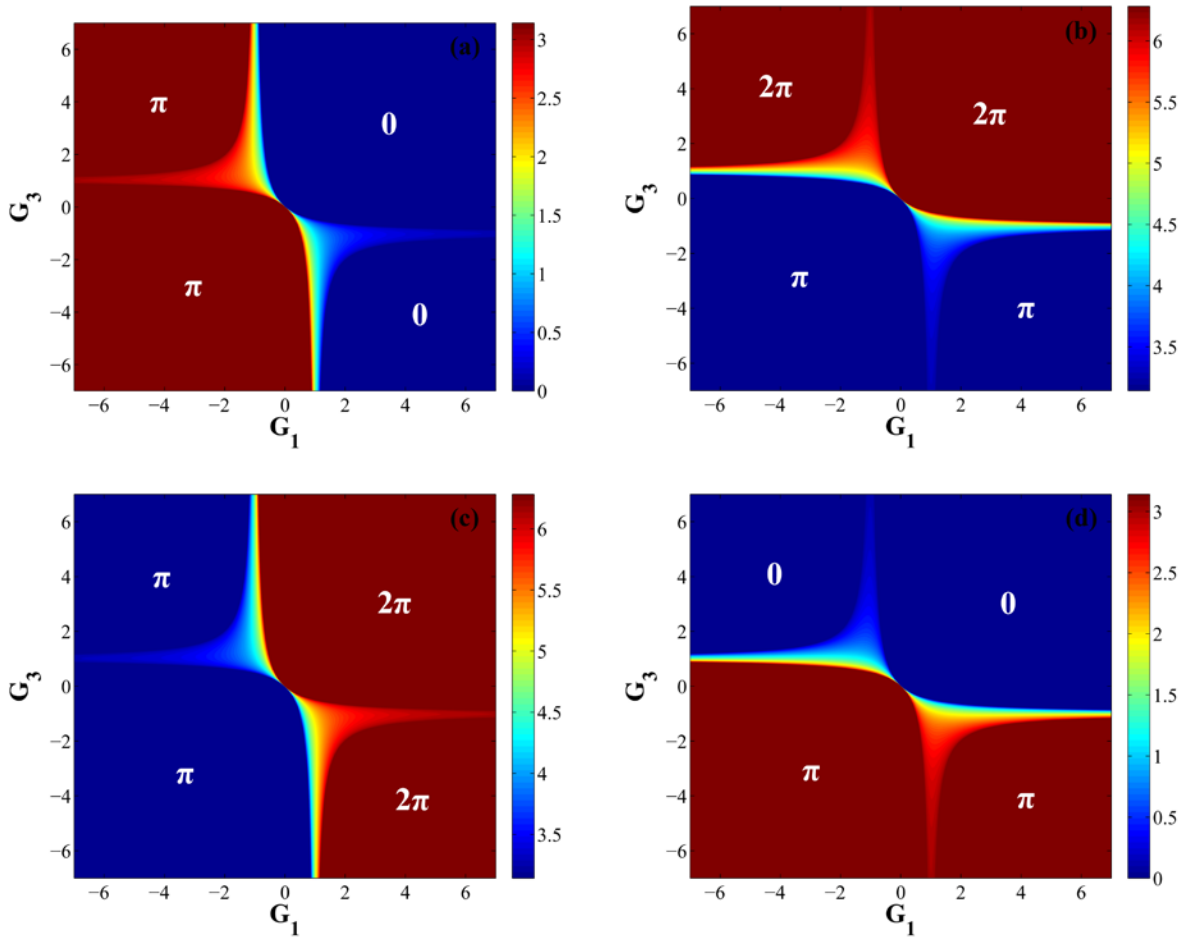


Fig. S2. The distribution of the phase differences $\phi$ (a, c) (left column) and $\theta$ (b, d) (right column) of the order parameters of a three-band superconductor with the set $G_2 = 1$. The top figures illustrate the combined solutions for one of the two-fold degenerate ground states. The bottom figures represent the combined solutions for the other second ground state.

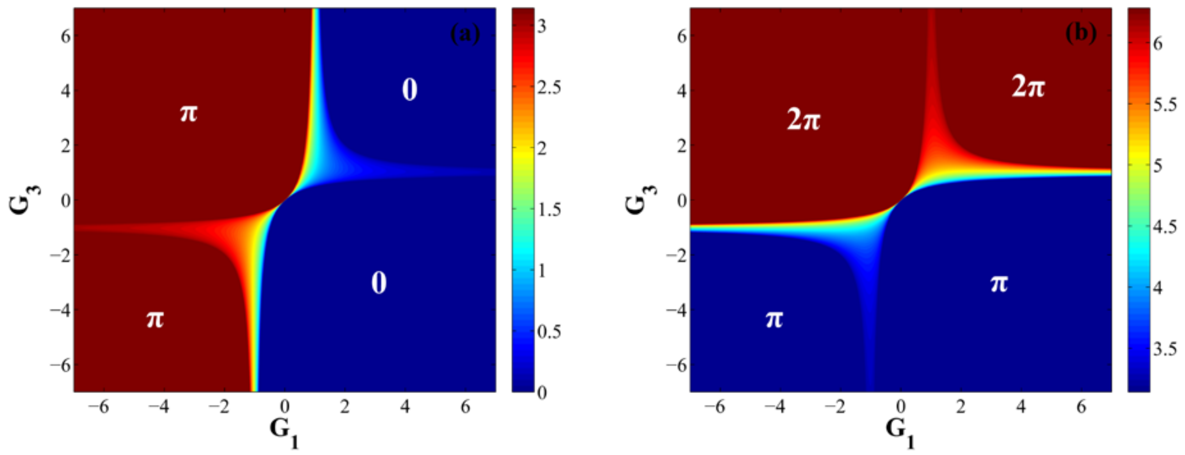

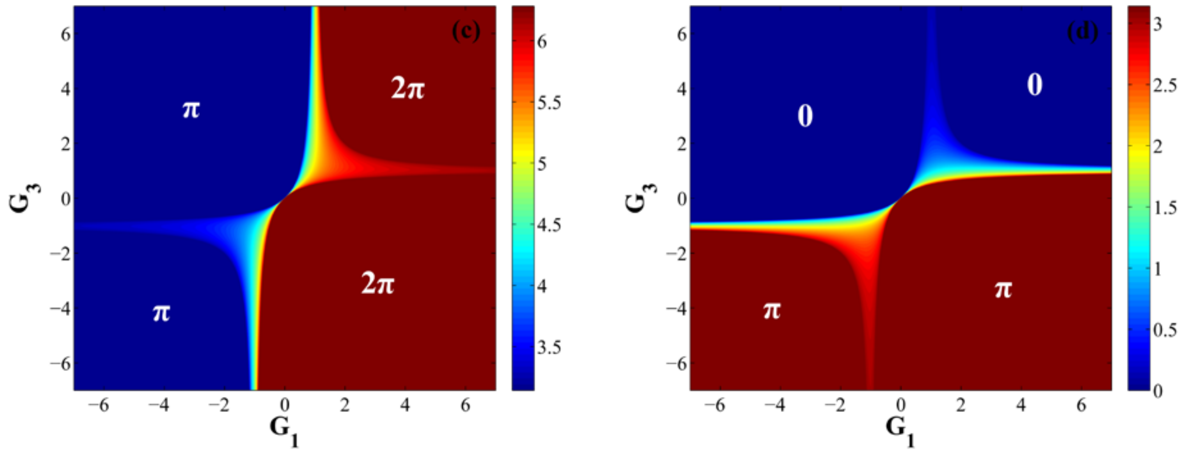


Fig. S3. The same as in Fig. S2 for the set $G_2 = -1$.

From Fig. 2 of the main text, Figs. S2, and S3, it becomes clear that the frequently found statement in the literature [1-8] that frustrated phase differences are realized for an odd number of repulsive interband interactions, only, is *not* fully correct. Frustration is realized only for relatively narrow intervals of $G_1$ and $G_3$ while for other values of the interband couplings (part of the $G_i$ coefficients) even in that case the twofold degeneracy of the ground state generic for frustration and BTRS can be removed in favor of a *single non-degenerate* ground state.

It's interesting to track the behavior of the interaction term $F_{\text{int}}$ of the GL free energy density functional versus $\phi$ and $\theta$ in dependence of $G_1$, $G_2$ and $G_3$. For this purpose we start with the BTRS case and restrict the values of $\phi$ and $\theta$ within the $[0, 2\pi]$ interval as it in the phase diagrams shown in Figs. S1 and S2.

Let's consider the set $G_i = \left(-1/2, 1, 1/\sqrt{3}\right)$. According to Eqs. (S13)-(S20) global maxima of $F_{\text{int}}$ (which correspond to global minima of the GL free energy) for this set $G_i$ are observed for $\phi = \pi/2$, $\theta = \pi/3$ and for $\phi = 3\pi/2$, $\theta = 5\pi/3$. This is also confirmed by inspecting the plot of the function $F_{\text{int}} = F_{\text{int}}(\phi, \theta)$ (Fig. S4 a, b). As we can see from the landscape there are one minimum at $\phi = 0$, $\theta = \pi$ and two saddle points at $\phi = \pi$, $\theta = \pi$ and $\phi = \pi$, $\theta = 0$.

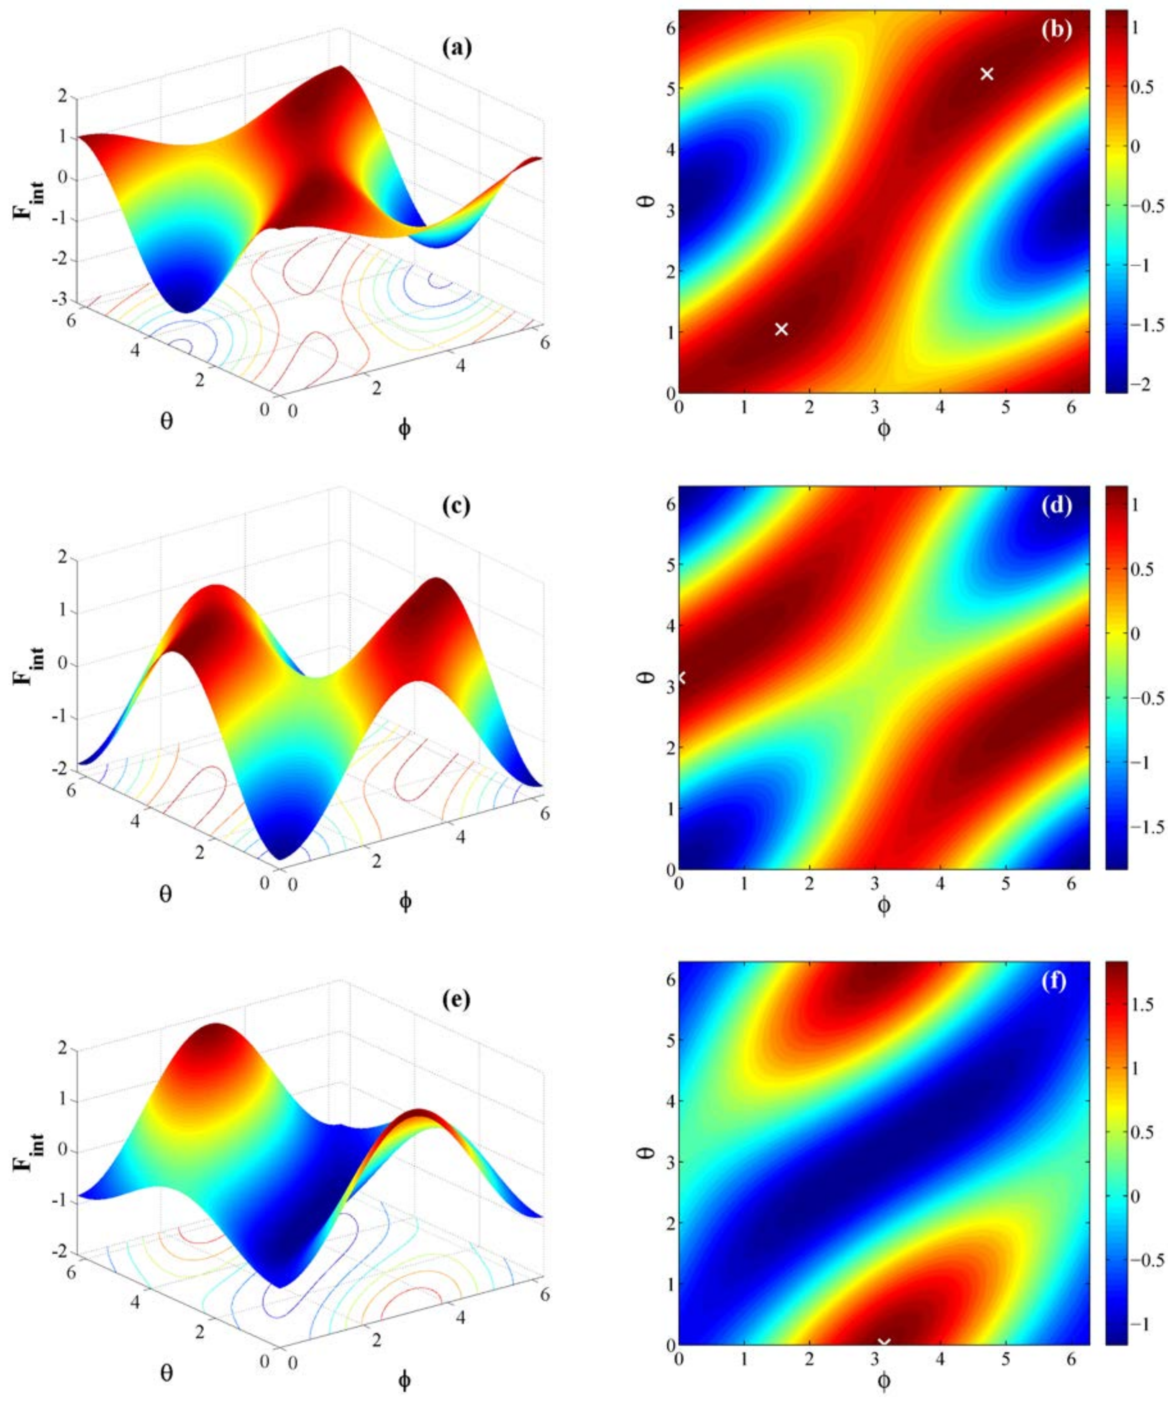

(a)
(b)
(c)
(d)
(e)
(f)
F_int
θ
ϕ

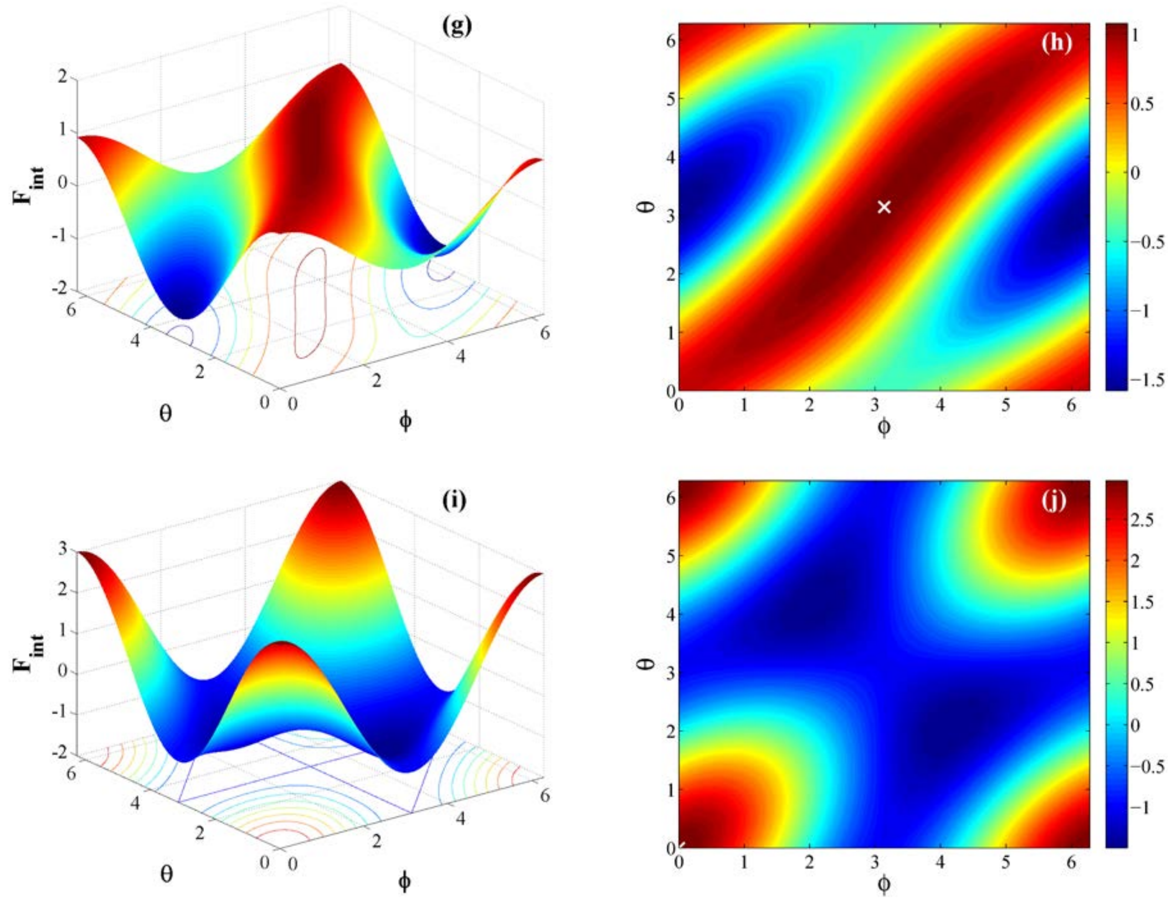


Fig. S4. The surface (left column) and the contour plot (right column) of the dependence of the interband interaction term $F_{\text{int}}$ of the GL free energy functional as a function of the phase differences for the sets $G_i = \left(-1/2, 1, 1/\sqrt{3}\right)$ (a, b), $G_i = \left(-1/3, -1, -1/2\right)$ (c, d), $G_i = \left(-1/3, -1, 1/2\right)$ (e, f), $G_i = \left(-1/3, 1, 1/4\right)$ (g, h) and $G_i = \left(1, 1, 1\right)$ (i, j). White crosses: global maxima of $F_{\text{int}}$ within the considered limited intervals of phase differences. .

The behavior of the interaction term for the "classical" BTRS case with $G_i = \left(1, -1, 1\right)$, where $\phi = \pi / 3$, $\theta = 5\pi / 3$ and $\phi = 5\pi / 3$, $\theta = \pi / 3$, is considered in the main paper (see fig. 1).

As we have already noted above not for all sets of $G_i$ frustration is realized. These corresponding non-degenerate states are realized when the phase differences equal to 0 or π. Moreover, for this situation we observe only a single ground state with conserved sign-reversal symmetry of the order parameter, i.e. a non-BTRS state. For instance, in Fig. S4 (c, d) the ground state at $\phi = 0$, $\theta = \pi$ with three (i.e. an odd number) of repulsive interband interactions is shown for $G_i = \left(-1/3, -1, -1/2\right)$, representing thereby a possible $s_{+\pm}$-wave symmetry of the order parameter. Also we can see from the figure S4 (c,d) a minimum for $\phi = 0$, $\theta = 0$ and two saddle points for $\phi = \pi$, $\theta = 0$ and $\phi = \pi$, $\theta = \pi$ .

A ground state with sign-reversal order parameters also takes place for $G_i = (-1/3, -1, 1/2)$ at $\phi = \pi, \theta = 0$ (Fig. S4e, f), where we get $s_{\pm+}$-wave symmetry. Note the presence of a minimum for $\phi = \pi$, $\theta = \pi$ and again two saddle points $\phi = 0$, $\theta = \pi$ and $\phi = 0$, $\theta = 0$. For the set with one (odd again) repulsive interband interaction $G_i = (-1/3, 1, 1/4)$ we observe a non-degenerated ground state at $\phi = \pi, \theta = \pi$ (Fig. S4 g, h) with an $s_{\pm-}$ order parameter. There are one minimum at $\phi = 0, \theta = \pi$ and two saddle points at $\phi = 0, \theta = 0$ and $\phi = \pi, \theta = 0$.

When all interband coefficients are positive (attractive interband interactions) we observe a single non-BTRS ground state at $\phi = 0$, $\theta = 0$ generic for the $s_{+++}$-wave symmetry. Figs. S4 (i, j) represent the behavior of the interaction term of the GL free energy density for $G_i = (1,1,1)$, where we have two minima at $\phi = 2\pi/3, \theta = 4\pi/3$ and $\phi = 4\pi/3, \theta = 2\pi/3$ together with three saddle points $\phi = \pi, \theta = \pi$, $\phi = 0, \theta = \pi$ and $\phi = \pi, \theta = 0$.

## 2. The Gibbs free energy functional

In view of the complete homogeneity of the system along the $z$ axis of the cylindrical coordinates, the Gibbs free-energy functional of a three-band superconductor takes the following form:

$$G = L\sum_i \int_{\Xi_s} \left[ \alpha_i |\psi_i|^2 + \frac{1}{2}\beta_i |\psi_i|^4 + \bar{\kappa}_i \left| \left( -i\hbar\nabla - \frac{2e}{c}\mathbf{A} \right)\psi_i \right|^2 \right] d^2\mathbf{r}$$

$$- L\int_{\Xi_s} \left[ \gamma_{12}\left(\psi_1^*\psi_2 + \psi_1\psi_2^*\right) + \gamma_{13}\left(\psi_1^*\psi_3 + \psi_3\psi_1^*\right) + \gamma_{23}\left(\psi_2^*\psi_3 + \psi_2\psi_3^*\right) \right] d^2\mathbf{r} + \frac{L}{8\pi}\int_{\Xi_s+\Xi_h} \left(\mathrm{rot}\,\mathbf{A} - \mathbf{H}\right)^2 d^2\mathbf{r} \tag{S24}$$

where the integration in the plane $(r, \vartheta)$ is carried out over the cross-section of the superconducting cylinder ($\Xi_s$), and over the cross-sections of the superconductor and of the open “hole” volume of the tube ($\Xi_s + \Xi_h$) in the last field term.

The expression for the current density has the form

$$j = -ie\hbar\sum_i \bar{\kappa}_i \left( \psi_i^*\nabla\psi_i - \psi_i\nabla\psi_i^* \right) - \frac{4e^2}{c}\mathbf{A}\sum_i \bar{\kappa}_i |\psi_i|^2 \tag{S25}$$

On the strength of conditions, formulated in the main paper (part III), $\mathrm{rot}\,\mathbf{A} \approx \mathbf{H}$ practically holds everywhere in the region $\Xi_h$ and the variations of $A_\vartheta(r)$ in $\Xi_s$ can be neglected. Taking these two facts into account and rewriting the order parameters as $\psi_i = |\psi_i| \exp(n\varphi_i(\vartheta))$, we get for the Gibbs free energy (S24)

$$\frac{G}{\pi R^2 L} = \sum_i \alpha_i |\psi_i|^2 + \frac{1}{2}\beta_i |\psi_i|^4 + \bar{\kappa}_i |\psi_i|^2 q^2 - 2\gamma_{12}|\psi_1||\psi_2|\cos\phi - 2\gamma_{13}|\psi_1||\psi_3|\cos\theta - 2\gamma_{23}|\psi_2||\psi_3|\cos(\theta-\phi)$$

(S26)

and the expression for the current density

$$j = 2e\hbar \sum_i \bar{\kappa}_i |\psi_i|^2 q\,. \tag{S27}$$

Here $q = \frac{1}{R}\left(n - \frac{\Phi}{\Phi_0}\right)$, where $\Phi = \pi R^2 H$ is the magnetic flux through the ring and $\Phi_0 = \frac{\pi\hbar c}{e}$ is the flux quantum.

## 3. BTRS in a mesoscopic ring imitating three-band superconductivity

Finally we consider briefly a mesoscopic system in the spirit of that imitating solitons in a two-band superconductor [9]. There two thin films of a conventional s-wave superconductor separated by a thin insulating film with intermediate Josephson coupling between them are considered. In our proposed mesoscopic ring there is also a Josephson coupling between the upper (conventional s-wave) and the lower (with an $s_\pm$ deposited superconducting material) ring as depicted in Fig. S5.

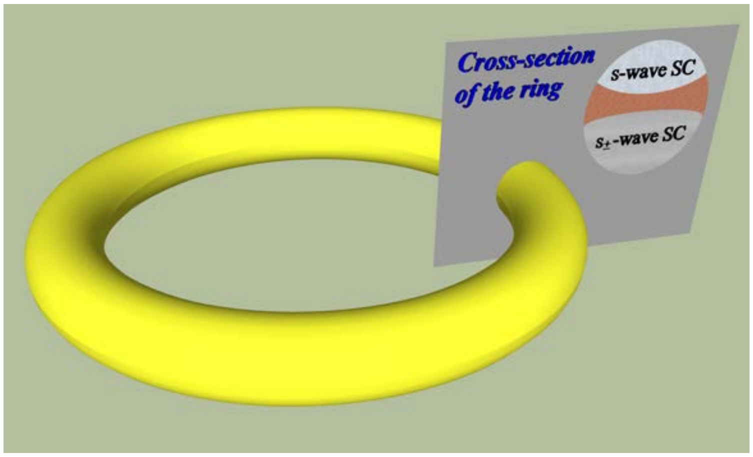


Fig. S5. (Color online) Schematical view of a mesoscopic ring with internal layered structure. The upper and the lower superconducting rings are supposed to be connected by a weak Josephson coupling due to the presence of an insulating middle ring (red) as shown schematically by the cross section of the torus in the upper right part of the figure.

This Josephson coupling causes the same chiral complex order parameter structure as considered in Sect. II in the main paper and this situation is well described by our adopted unrestricted Ginzburg-Landau aproach. Thereby the inhomogeneous case with phase solitons to be

considered elsewhere in the spirit of Ref. 10 must be applied. Since this is already beyond the scope of the present paper, a more detail description will be given also elsewhere.

## References


1. T. A. Bojesen, E. Babaev, and A. Sudbø, Phys. Rev. B **88**, 220511 (2013).
2. V. Stanev and Z. Tesanovic, Phys. Rev. B **81**, 134522 (2010).
3. Y. Tanaka and T. Yanagisawa, J. Phys. Soc. Jpn. **79**, 114706 (2010).
4. Y. Tanaka and T. Yanagisawa, Solid State Com., **150**, 1980 (2010)
5. R. G. Dias and A. M. Marques, Superconductor Science and Technology **24**, 085009 (2011)
6. J. Garaud, J. Carlstrom, and E. Babaev, Phys. Rev. Lett. **107**, 197001 (2011).
7. V. Stanev, Phys. Rev. B **85**, 174520 (2012).
8. J. Garaud, J. Carlstrom, E. Babaev, and M. Speight, Phys. Rev. B **87**, 014507 (2013).
9. H. Bluhm, N. Koshnik, M. Huber, and K. Moler, Phys. Rev. Lett. 97, 237002 (2005).
10. S. V. Kuplevakhsky, A. N. Omelyanchouk, and Y. S. Yerin, Low Temp. Phys. 37, 667 (2011).
